# Supplementary material for: Provably Stable Flux Reconstruction High-Order Methods on Curvilinear Elements
Source: arXiv:2109.11617 source file (2021-09-23)
Supplement: Supplementary file 1 [file Curv_grid_choice.tex]

\iffalse

\section{On the Choice of Curvilinear Grids}

-This section \cite{mengaldo2016connections} grid put energy results and talk about the importance of choice of grid

\begin{equation}
\begin{split}
    \frac{\partial u}{\partial t} + \frac{\partial u}{\partial x} +\frac{\partial u}{\partial y} = 0,\\
    u(x,y,0) = e^{-20(x^2+y^2)}
    \end{split}
\end{equation}

 \begin{table}[t]
\resizebox{\textwidth}{!}{
%\begin{center} 
 \begin{tabular}{c c c c }
Scheme &  Flux & Energy Conserved $\mathcal{O}$(1e-12) & Energy Monotonically Decrease \\ \hline 
Cons. DG & Central & \textbf{Yes} & \textbf{Yes} \\ \hline 
Cons. DG & Upwind & No& \textbf{Yes} \\ \hline 
EFSR Split $c_{DG}$ & Central & \textbf{Yes} & \textbf{Yes} \\ \hline 
EFSR Split $c_{DG}$ & Upwind & No & \textbf{Yes} \\ \hline 
EFSR Split $c_{+}$ & Central  & \textbf{Yes} &\textbf{Yes} \\ \hline 
EFSR Split $c_{+}$ & Upwind &No & \textbf{Yes} \\ \hline 
EFSR Classical Split $c_{+}$ & Central  &\textbf{Yes} & \textbf{Yes} \\ \hline 
EFSR Classical Split $c_{+}$ & Upwind & No & \textbf{Yes} 
\end{tabular} 
 %\end{center} 
 }
 \caption{Energy Results $p=3,4$ Uncollocated $N_{vp}=(p+1)^2$ Symmetric Grid} 
 \label{tab:grid 1 stability}
 \end{table} 
 
 \fi
